# Supplementary material for: Search for the Standard Model Higgs Boson Produced in Association with a $W$ Boson in the Isolated-Track Charged-Lepton Channel Using the Collider Detector at Fermilab
Source: arXiv:1110.5349 source file (2011-10-24)
Supplement: Supplementary file 1 [file controlPlots_BNN_PretagSVTSVT_CEMCMUPCMX.tex]

%\clearpage

%%% For BNN PretagSVTSVT TIGHT charged lepton %%%

% BNN inputs 1/3
\begin{figure}[ht]
  \begin{center}
    \includegraphics[width=6.6cm]{./appendix/ControPlots/Kinematics/WH_PretagSVTSVT_CEMCMUPCMX_Mj1j2Corr.eps}
    \includegraphics[width=6.6cm]{./appendix/ControPlots/KinematicsLog/WH_PretagSVTSVT_CEMCMUPCMX_Mj1j2Corr.eps}
    \includegraphics[width=6.6cm]{EPSfigure_5.7fb/Kinematics/WH_PretagSVTSVT_CEMCMUPCMX_ptImbal.eps}
    \includegraphics[width=6.6cm]{EPSfigure_5.7fb/KinematicsLog/WH_PretagSVTSVT_CEMCMUPCMX_ptImbal.eps}
    \includegraphics[width=6.6cm]{EPSfigure_5.7fb/Kinematics/WH_PretagSVTSVT_CEMCMUPCMX_qEta.eps}
    \includegraphics[width=6.6cm]{EPSfigure_5.7fb/KinematicsLog/WH_PretagSVTSVT_CEMCMUPCMX_qEta.eps}
    \caption {TIGHT charged lepton Pretag BNN Input Kinematics}
  \end {center}
\end {figure}

% BNN inputs 2/3
\begin{figure}[ht]
  \begin{center}
    \includegraphics[width=6.6cm]{EPSfigure_5.7fb/Kinematics/WH_PretagSVTSVT_CEMCMUPCMX_minMlnb.eps}
    \includegraphics[width=6.6cm]{EPSfigure_5.7fb/KinematicsLog/WH_PretagSVTSVT_CEMCMUPCMX_minMlnb.eps}
    \includegraphics[width=6.6cm]{EPSfigure_5.7fb/Kinematics/WH_PretagSVTSVT_CEMCMUPCMX_maxMlnb.eps}
    \includegraphics[width=6.6cm]{EPSfigure_5.7fb/KinematicsLog/WH_PretagSVTSVT_CEMCMUPCMX_maxMlnb.eps}
    \includegraphics[width=6.6cm]{EPSfigure_5.7fb/Kinematics/WH_PretagSVTSVT_CEMCMUPCMX_sumLooseJetEt.eps}
    \includegraphics[width=6.6cm]{EPSfigure_5.7fb/KinematicsLog/WH_PretagSVTSVT_CEMCMUPCMX_sumLooseJetEt.eps}
    \caption {TIGHT charged lepton Pretag BNN Input Kinematics}
  \end {center}
\end {figure}

% BNN inputs 3/3
\begin{figure}[ht]
  \begin{center}
    \includegraphics[width=6.6cm]{EPSfigure_5.7fb/Kinematics/WH_PretagSVTSVT_CEMCMUPCMX_wPt.eps}
    \includegraphics[width=6.6cm]{EPSfigure_5.7fb/KinematicsLog/WH_PretagSVTSVT_CEMCMUPCMX_wPt.eps}
    \includegraphics[width=6.6cm]{EPSfigure_5.7fb/Kinematics/WH_PretagSVTSVT_CEMCMUPCMX_ht.eps}
    \includegraphics[width=6.6cm]{EPSfigure_5.7fb/KinematicsLog/WH_PretagSVTSVT_CEMCMUPCMX_ht.eps}
    \includegraphics[width=6.6cm]{EPSfigure_5.7fb/Kinematics/WH_PretagSVTSVT_CEMCMUPCMX_met.eps}
    \includegraphics[width=6.6cm]{EPSfigure_5.7fb/KinematicsLog/WH_PretagSVTSVT_CEMCMUPCMX_met.eps}
    \caption {TIGHT charged lepton Pretag BNN Input Kinematics}
  \end {center}
\end {figure}

% BNN outputs 1/4
\begin{figure}[ht]
  \begin{center}
    \includegraphics[width=6.6cm]{EPSfigure_5.7fb/Kinematics/WH_PretagSVTSVT_CEMCMUPCMX_bnn_wh100.eps}
    \includegraphics[width=6.6cm]{EPSfigure_5.7fb/KinematicsLog/WH_PretagSVTSVT_CEMCMUPCMX_bnn_wh100.eps}
    \includegraphics[width=6.6cm]{EPSfigure_5.7fb/Kinematics/WH_PretagSVTSVT_CEMCMUPCMX_bnn_wh105.eps}
    \includegraphics[width=6.6cm]{EPSfigure_5.7fb/KinematicsLog/WH_PretagSVTSVT_CEMCMUPCMX_bnn_wh105.eps}
    \includegraphics[width=6.6cm]{EPSfigure_5.7fb/Kinematics/WH_PretagSVTSVT_CEMCMUPCMX_bnn_wh110.eps}
    \includegraphics[width=6.6cm]{EPSfigure_5.7fb/KinematicsLog/WH_PretagSVTSVT_CEMCMUPCMX_bnn_wh110.eps}
    \caption {TIGHT charged lepton Pretag BNN Outputs Kinematics (using SVTSVT BNN)}
  \end {center}
\end {figure}

% BNN outputs 2/4
\begin{figure}[ht]
  \begin{center}
    \includegraphics[width=6.6cm]{EPSfigure_5.7fb/Kinematics/WH_PretagSVTSVT_CEMCMUPCMX_bnn_wh115.eps}
    \includegraphics[width=6.6cm]{EPSfigure_5.7fb/KinematicsLog/WH_PretagSVTSVT_CEMCMUPCMX_bnn_wh115.eps}
    \includegraphics[width=6.6cm]{EPSfigure_5.7fb/Kinematics/WH_PretagSVTSVT_CEMCMUPCMX_bnn_wh120.eps}
    \includegraphics[width=6.6cm]{EPSfigure_5.7fb/KinematicsLog/WH_PretagSVTSVT_CEMCMUPCMX_bnn_wh120.eps}
    \includegraphics[width=6.6cm]{EPSfigure_5.7fb/Kinematics/WH_PretagSVTSVT_CEMCMUPCMX_bnn_wh125.eps}
    \includegraphics[width=6.6cm]{EPSfigure_5.7fb/KinematicsLog/WH_PretagSVTSVT_CEMCMUPCMX_bnn_wh125.eps}
    \caption {TIGHT charged lepton Pretag BNN Outputs Kinematics (using SVTSVT BNN)}
  \end {center}
\end {figure}

% BNN outputs 3/4
\begin{figure}[ht]
  \begin{center}
    \includegraphics[width=6.6cm]{EPSfigure_5.7fb/Kinematics/WH_PretagSVTSVT_CEMCMUPCMX_bnn_wh130.eps}
    \includegraphics[width=6.6cm]{EPSfigure_5.7fb/KinematicsLog/WH_PretagSVTSVT_CEMCMUPCMX_bnn_wh130.eps}
    \includegraphics[width=6.6cm]{EPSfigure_5.7fb/Kinematics/WH_PretagSVTSVT_CEMCMUPCMX_bnn_wh135.eps}
    \includegraphics[width=6.6cm]{EPSfigure_5.7fb/KinematicsLog/WH_PretagSVTSVT_CEMCMUPCMX_bnn_wh135.eps}
    \includegraphics[width=6.6cm]{EPSfigure_5.7fb/Kinematics/WH_PretagSVTSVT_CEMCMUPCMX_bnn_wh140.eps}
    \includegraphics[width=6.6cm]{EPSfigure_5.7fb/KinematicsLog/WH_PretagSVTSVT_CEMCMUPCMX_bnn_wh140.eps}
    \caption {TIGHT charged lepton Pretag BNN Outputs Kinematics (using SVTSVT BNN)}
  \end {center}
\end {figure}

% BNN outputs 4/4
\begin{figure}[ht]
  \begin{center}
    \includegraphics[width=6.6cm]{EPSfigure_5.7fb/Kinematics/WH_PretagSVTSVT_CEMCMUPCMX_bnn_wh145.eps}
    \includegraphics[width=6.6cm]{EPSfigure_5.7fb/KinematicsLog/WH_PretagSVTSVT_CEMCMUPCMX_bnn_wh145.eps}
    \includegraphics[width=6.6cm]{EPSfigure_5.7fb/Kinematics/WH_PretagSVTSVT_CEMCMUPCMX_bnn_wh150.eps}
    \includegraphics[width=6.6cm]{EPSfigure_5.7fb/KinematicsLog/WH_PretagSVTSVT_CEMCMUPCMX_bnn_wh150.eps}
    \caption {TIGHT charged lepton Pretag BNN Outputs Kinematics (using SVTSVT BNN)}
  \end {center}
\end {figure}
